# Supplementary material for: Preservation of scalar spin chirality across a metallic spacer in synthetic antiferromagnets with chiral interlayer interactions
Source: arXiv:2404.07637 source file (2024-05-10)
Supplement: Supplementary file 1 [file supplementary.tex]

In this section, the magnetic states forming in the SAF described in section \ref{sec:saf_description} are investigated with XRR for both OOP configurations of the Co layer ($+m_{z}$ and $-m_{z}$). Experiments took place at SEXTANTS beamline of SOLEIL synchrotron \cite{sacchi2013sextants}. The OOP fields required to saturate the Co layer are significantly large ($>$ 250 mT) due to its strong PMA \cite{fernandez2019symmetry}, thus the initialization was performed outside of the RESOXS chamber by perpendicularly approaching a strong permanent magnet (350 mT) against the sample's surface, as sketched in figure \ref{fig:xrms_mounting} (a). The sample was then mounted in the holder with the nominal EA parallel to the X-ray beam (experimental geometry shown in figure \ref{fig:xrms_mounting} (b)).

Prior to the $\theta$-2$\theta$ XRR scan experiments, a series of measurements were taken to calibrate the beamline and find the optimal experimental conditions. For this, energy scans were performed in order to find the absorption edges' energies, with the CoFeB layer fully saturated along $+m_{x}$ and the Co layer along $-m_{z}$, at $\theta = 15^{\circ}$ of incidence with respect to the surface plane, which gives large sensitivity to IP magnetization \cite{jal2013reflectivite}. The scans shown in figures \ref{fig:ch3f2} (a,b) represent the XMCD or dichroic signal which is computed via the asymmetry ratio, expression \ref{eq:xmcd}, with $I_{\text{CL}}$ and $I_{\text{CR}}$ in this case being respectively the XRR signals measured for CL and CR incident polarization in the vicinity of the Fe and Co's absorption edges. The energies at the highest peaks ($L_{3}$-edge) are found at 709.5 and 784.0 eV respectively, given by the vertical red dashed-lines.

Figure \ref{fig:ch3f2} (c) shows an XRR scan for both circular incident polarizations, taken at the Fe-edge with the CoFeB saturated along $+m_{x}$, and the Co layer saturated along $+m_{z}$. The intensity profiles are plotted on logarithmic scale, given the very strong dependence between reflectivity and incidence angle. Its corresponding XMCD signal is given by the blue curve in figure \ref{fig:ch3f2} (d). The other curves show XMCD profiles for different XRR measurements under different magnetic configurations, as described by the legend captions.

When measuring at the Fe-edge only sensitivity to the magnetic state of the CoFeB layer is achieved, hence, the blue and green curves should theoretically be identical given that the CoFeB layer holds the same magnetic state ($+m_{x}$). However, this does not occur, the discrepancies observed between them could be due to slightly different magnetic states in the CoFeB layer, or other unknown effects. Differently, when the X-ray energy is tuned to the Co-edge, the reflected beam gives simultaneous sensitivity to both CoFeB and Co layers' magnetic configurations. The differences observed between the orange and red curves are due to an oppositely polarized Co layer, in addition to the previously mentioned possible difference in CoFeB state. The out of resonance (OOR) measurement (always at 690 eV), represented by the purple curve, gives a flat XMCD signal as expected.

XRR has been used to quantitatively determine the configuration of the magnetic layers, by fitting the reflectivity curve as a function of the incidence angle to an analytical model. The formalism is explained in\cite{elzo2012x}, where each of the layers is individually modeled properly taking into account the different interfaces involved. In this particular case, obtaining meaningful information has proven to be very difficult. The reason for this is that the layers show significant roughness as evidenced by the cross section measurement shown in figure \ref{fig:cross_sect}, which was taken by Dr. Damien McGrouther at the University of Glasgow using a JEOL ARM200CF TEM microscope. This long-range roughness and layer inter-mixing can not be properly described by the analytical model.

Given that no clear conclusions can be drawn from these measurements, in the following section, a different approach is followed utilizing the X-ray technique described in section \ref{sec:xmcdchirality}.

\section{Determination of chiral spin states via diffuse scattering analysis}\label{sec:diff_scatt}

For these experiments, the point detector described in section \ref{sec:xrms} is replaced by a CCD camera which provides a spatially resolved diffuse magnetic scattering map, \textit{i.e.}, an XRMS map. By analysis of the off-specular components in combination with the theoretical framework described in section \ref{sec:xmcdchirality}, the formation of chiral magnetic structures is investigated in Fourier-space.

\section{Atomistic/effective field sims}

In this section, two different models which describe the IL-DMI effect are utilized to explain the experimental findings discussed in the preceding sections. First, describing IL-DMI via the atomistic model explained in\cite{vedmedenko2019interlayer}, and then as an effective unidirectional IP field related with the orientation of the Co layer\cite{han2019long}.

Here, the atomistic model described in\cite{vedmedenko2019interlayer} is applied to ideal 1D 180$^{\circ}$ DWs, evaluating the IL-DMI energy for all possible combinations of CoFeB IP chirality and OOP orientation of the Co layer, summarized in figure . These simulations were performed with the support of our collaborator Dr. Elena Vedmedenko.

Figures (a,b) represent two opposite IP chiral 180$^{\circ}$ head-to-head DWs forming in the CoFeB, \textit{i.e.}, counter-clockwise (CCW) and clockwise (CW), and figures (c,d) and (e,f) correspond respectively to the IL-DMI energies for both Co OOP orientations. The DW IL-DMI energy profile is clearly asymmetric; the core of the DW is opposite in energy to the outer part, which implies that indeed IL-DMI creates asymmetries in the energy landscape of 180$^{\circ}$ DWs. The IL-DMI changes sign upon reversal of the Co layer, and also with inverting the CoFeB IP chirality, which qualitatively agrees with experiments.

Nevertheless, if the same combinations are performed after reversing the $\hat{x}$ component of the domains as in figure , \textit{i.e.}, tail-to-tail DWs going from $-m_{x}$ to $+m_{x}$, the energy profiles contradict the experimental findings. There is no link between IL-DMI energy and chirality, but rather between IL-DMI and sign of the 180$^{\circ}$ DW $\hat{y}$ component. That is the reason why the profiles sketched in figures  (a) and  (a) which have the same chirality but different $\hat{y}$ component, give opposite IL-DMI energies (likewise for figures (b) and  (b)) for the same Co orientations.

The atomistic model thus explains the asymmetry during the reversal observed in\cite{fernandez2019symmetry}, and also evidences a clear asymmetry in the energetic configuration of 180$^{\circ}$ DWs, but fails in linking directly with IP chirality as the XRMS maps from experiments suggest. It is investigated in the next section if a unidirectional effective field, as modeled in\cite{han2019long}, could explain the effect.

In order to assess whether IL-DMI as an effective unidirectional field\cite{han2019long} would explain the chirality dependent experimental results, an approach that combines an effective field with other energy interactions present in the samples is followed. For this, the start-point consists of assuming for the CoFeB layer the configuration shown in figure(a), \textit{i.e.}, a circular domain separated by 180$^{\circ}$ DWs, whose components are initially left as unknowns for assessing which configuration is most probable. Now, the effect of intralayer DMI is included, which in thin films promotes Néel DWs with OOP component given by the symbols in figure  (b). For an IP dominated film, this would add certain OOP DW component with the sign given by the symbols, leaving a canted magnetic state. In this case, an OOP CW sense of rotation along the dashed line is assumed. If now antiferromagnetic RKKY coupling with the fully OOP Co layer is included, a particular side of the DW will be unfavored whereas the other will be favored, and vice-versa upon reversal of the Co layer. This effect is sketched in figures  (c,d) for both possible OOP orientations of the Co, making narrower or wider respectively the unfavored or favored DW components.

Now, the unidirectional effective field along the EA due to IL-DMI () is added on top of the Co dependent asymmetric DW width. In this model, for Co layer magnetized along $+m_{z}$, \textit{i.e.}, coming out of the page as in figures  (a,b), $\Vec{B}_{\text{IL-DMI}}$ on the CoFeB is assumed to lie along $+m_{x}$. Differently, when Co is magnetized oppositely along $-m_{z}$, $\Vec{B}_{\text{IL-DMI}}$ flips 180$^{\circ}$ and lies along $-m_{x}$.

In order to link with experiments, an external magnetic field $\Vec{B}_{ext}$ is added to compensate $\Vec{B}_{\text{IL-DMI}}$. Two different approaches are followed; first, $\Vec{B}_{ext}$ is applied perfectly along the EA direction giving zero net $\hat{y}$ field component, compensating perfectly $\Vec{B}_{\text{IL-DMI}}$. In this case, none of the fields break the symmetry along the $\hat{y}$ direction, hence, any configuration of $m_{y}$ giving net chiral or achiral (AC) magnetic configurations along the dashed line is equally probable regardless of the orientation of the Co layer. This approach does not explain the observed results.

Differently, if $\Vec{B}_{ext}$ has a non-zero $\hat{y}$ component due to misalignment between the electromagnet and anisotropy axis, as it would be likely to occur experimentally, results are different. In figure  (b), $\Vec{B}_{ext}$'s $\hat{x}$ component fully compensates $\Vec{B}_{\text{IL-DMI}}$, leaving a net $-\hat{y}$ component. In this case not all DW configurations are equally probable as in figures  (a,c); the most likely DW components are determined by both the sign of the transverse component of the net field acting on the texture and the width of the DW due to the intralayer DMI and RKKY coupling. Thus, the most probable configuration (1) is for both wide and narrow DW components to have the sign of the net field. The next most probable state (2) is for the wider DW to be parallel to the transverse field whereas the narrow is magnetized oppositely (given that the area is larger). The third state (3) corresponds to the narrow area magnetized along the field direction and the wide area opposite to the net field, and the least likely case (4) is where both narrow and wide DWs are magnetized opposite to the field.

Reversing the orientation of the Co layer, and consequently the bias field, changes the sign of the exchange bias. To compensate for this, the sign of both $\hat{x}$ and $\hat{y}$ components of $\Vec{B}_{ext}$ also need to be inverted, leaving as a consequence a net $+\hat{y}$ component as evidenced in the inset of figure \ref{fig:energy_probs} (d). However, it can be observed that the most probable configurations have the same probability regardless of the Co orientation; in both cases of figures \ref{fig:energy_probs} (c,d), the achiral configuration is the most likely, followed by clockwise and counter-clockwise rotations, and at last the other achiral state. Thus, modelling IL-DMI as an effective field in combination with other energies present in the SAF, does not reproduce the chirality dependent experimental results shown in section \ref{sec:diff_scatt}.
